# Supplementary material for: Controlling magnetoresistance by tuning semimetallicity through dimensional confinement and heteroepitaxy
Source: arXiv:2002.06167 ancillary file (2022-01-05)
Supplement: Supplementary file 1 [file SupplementaryInformation.pdf]

# Supplemental Material: Controlling magnetoresistance by tuning semimetallicity through dimensional confinement and heteroepitaxy

Shouvik Chatterjee,<sup>1,2,\*</sup> Shoaib Khalid,<sup>3,4</sup> Hadass S. Inbar,<sup>5</sup> Aranya Goswami,<sup>1</sup> Taozhi Guo,<sup>6</sup> Yu-Hao Chang,<sup>5</sup> Elliot Young,<sup>5</sup> Alexei V. Fedorov,<sup>7</sup> Dan Read,<sup>1,8</sup> Anderson Janotti,<sup>4,\*</sup> and Christopher J. Palmström<sup>1,5,\*</sup>

<sup>1</sup>*Department of Electrical & Computer Engineering,  
University of California, Santa Barbara, CA 93106, USA*

<sup>2</sup>*Present Address: Tata Institute of Fundamental Research, Homi Bhabha Road, Mumbai 400005, India*

<sup>3</sup>*Department of Physics and Astronomy, University of Delaware, Newark, DE 19716, USA*

<sup>4</sup>*Department of Materials Science and Engineering,  
University of Delaware, Newark, DE 19716, USA*

<sup>5</sup>*Materials Department, University of California, Santa Barbara, CA 93106, USA*

<sup>6</sup>*Department of Physics, University of California, Santa Barbara, CA 93106, USA*

<sup>7</sup>*Advanced Light Source, Lawrence Berkeley National Laboratory, Berkeley, California 94720, USA*

<sup>8</sup>*School of Physics and Astronomy, Cardiff University, Cardiff CF24 3AA, UK*

(Dated: October 14, 2020)

---

\* Authors to whom correspondence should be addressed: shouvik.chatterjee@tifr.res.in, cjpalm@ucsb.edu, janotti@udel.edu

## I. THIN FILM GROWTH AND ESTIMATION OF FILM THICKNESS:

Epitaxial thin films of LuSb were synthesized by molecular-beam epitaxy (MBE) in MOD Gen II growth chamber at 350°C by co-depositing Lu and Sb from Langmuir effusion cells with the Lu to Sb flux ratio set at 1:1.1. Samples of different thicknesses were grown under the same conditions on the same day. Prior to LuSb growth, 5nm thick GaSb buffer layer was grown at 450°C under Sb<sub>4</sub> overpressure on low n-type doped (001) GaSb substrates that freezes out at low temperatures. Native oxide was desorbed from GaSb substrates using atomic hydrogen. Before growth, atomic fluxes of Lu and Sb were determined by *in-situ* beam flux measurements using an ion gauge that allowed us to synthesize thin films of different nominal thicknesses by adjusting the growth time. Beam flux measurements were calibrated by Rutherford backscattering spectrometry (RBS) by measuring the elemental area density of calibration samples on Si. Sample surfaces were protected by a 5nm thick AlO<sub>x</sub> layer deposited *in vacuo* using e-beam evaporation before taking the samples out of the UHV chamber. For the ARPES measurements conductive n-type Te doped GaSb (001) substrates were used.

To confirm the thickness of our thin films we utilized Laue oscillations around the LuSb (002) diffraction peak, shown in Fig. S1. Theoretical x-ray spectrum for the Laue oscillations is given by

$$I = \frac{\sin^2(\pi N a \sin\theta/\lambda)}{\sin^2(\pi a \sin\theta/\lambda)} \quad (\text{S1})$$

where  $N$  is the number of monolayers,  $a$  is the LuSb lattice constant, and  $\lambda$  is the wavelength of the Cu K- $\alpha$  x-ray radiation used for the study. Calculated spectrum for the 40 and 20ML thick films is shown in Figs. S1A,B. showing excellent correspondence with the experimental data.

## II. EXTRACTION OF FERMİ WAVEVECTOR AND EFFECTIVE MASS CALCULATION

Both Fermi wavevector and Fermi velocity is obtained from a linear fit of the band dispersion along  $\bar{M} - \Gamma - \bar{M}$  close to the Fermi level within an energy range of 100 meV, measured using angle-resolved photoemission spectroscopy (ARPES). The band dispersion is extracted from the momentum-distribution curves (MDCs). Extracted band dispersion and the corresponding linear fits are shown in Fig. S2.

## III. ESTIMATION OF EFFECTIVE MASS AND QUANTUM MOBILITY

Quantum oscillations were observed in the 40, 32 and 20ML thick films. To reliably extract effective mass and quantum mobility in the multi-band compound, LuSb, oscillations corresponding to individual frequencies were obtained by the application of inverse Fourier transform on individual frequencies extracted using a band-pass filter on the fast Fourier transform data from the whole film, shown in Fig. 1F in the main text. According to the Lifshitz-Kosevich formula

$$\frac{\Delta R}{R(0)} \propto R_T R_H R_S \cos[2\pi(\frac{f}{\mu_0 H} - \gamma - \delta)] \quad (\text{S2})$$

where  $R_T$ ,  $R_H$ , and  $R_S$  are temperature, field, and the spin dependent damping factors. Effective mass is calculated from the temperature dependent damping of the oscillation amplitude at a particular magnetic field given by

$$R_T = \frac{(2\pi^2 k_B m^* T / e \hbar \mu_0 H)}{\sinh(2\pi^2 k_B m^* T / e \hbar \mu_0 H)}. \quad (\text{S3})$$

Field-dependent damping parameter  $R_H$  in Eq. S2 is given by

$$R_H = e^{-\pi/\mu_q \mu_0 H}, \quad (\text{S4})$$

where  $\mu_q$  is the quantum mobility. Thus, once  $m^*$  is determined using Eq. S3 (shown in Fig. S3A-C), assuming  $R_S$  is independent of magnetic field,  $\mu_q$  can be determined from the slope of  $\ln(\frac{\Delta R}{R(0)} \times 1/R_T)$  plotted against  $1/\mu_0 H$ , as shown in Fig. S3D-J

#### IV. COMPUTATIONAL APPROACH AND ADDITIONAL RESULTS OF THE DFT CALCULATIONS

Our first-principles calculations are based on the density functional theory (DFT) and projector augmented wave (PAW)<sup>1</sup> method as implemented in the VASP code.<sup>2,3</sup> For the exchange and correlation we employed both the generalized gradient approximation (GGA) of Perdew-Burke-Ernzerhof<sup>4</sup> and the screened hybrid functional (HSE06).<sup>5,6</sup> The exchange potential in HSE06 is divided into short range and long range parts separated by a screening parameter of  $\omega = 0.20 \text{ \AA}^{-1}$ . In the short range part the Hartree-Fock exchange and the GGA exchange are mixed with a ratio 25:75. In the long range part only the GGA exchange is used. The PAW potential for Sb contains five valence electrons,  $5s^2 5p^3$ , and for Lu, it contains 9 valence electrons,  $5p^6 6s^2 5d^1$ . The inclusion of the localized  $4f$  orbitals in Lu shows up as a dispersionless band at around 8 eV below the Fermi level with less than 5% change in carrier concentration based on test calculations. The effects of spin-orbit coupling (SOC) are included in all calculations.

The calculated DFT-GGA and HSE06 electronic band structures of bulk LuSb using the tetragonal cell with 4 atoms, corresponding to the smallest cell that can represent the (001) surface of LuSb, are shown in Fig. S6. These calculations were performed using an  $8 \times 8 \times 6$   $\Gamma$ -centered mesh of special  $k$ -points. As recently reported,<sup>7</sup> we find that the GGA functional overestimates the overlap between the electron and hole pockets, in analogy to the well-known underestimation of band gap in semiconductors and insulators. This overestimation leads to higher carrier concentrations and larger Fermi wavevectors when using the DFT-GGA functional, while the HSE06 functional gives results in very good agreement with the experimental data.<sup>8</sup> In order to compare the calculated Fermi wavevector ( $k_F$ ) with the ARPES data we scaled DFT-GGA to HSE06 results. This scaling shows good agreement with the experiment, as displayed in Fig. 3 in the main text.

The DFT-GGA calculations for LuSb (001) slabs with 7, 13, 21, and 41ML are shown in Fig. S7. These calculations were carried out using a  $12 \times 12 \times 1$  special  $k$ -points, and the Fermi level was used as a reference in the energy axis. HSE06 calculations for these slabs are prohibitively expensive given the size of the supercell and the large number of  $k$ -points required to describe metallic systems. The electron pocket at  $\bar{\Gamma}$  seen in the bulk (Fig. S6) and in the surface band structures (Fig. S7) are projections of the pockets at  $X_3$  in the bulk primitive cell (2 atoms/per cell) that is folded to  $\bar{\Gamma}$  in the bulk when using the 4-atom tetragonal unit cell and the slab calculations.

From Fig. S7 we can see that the electron pocket at  $\bar{\Gamma}$  is strongly affected by quantum confinement, contrary to the experimental data shown in Fig. 2,3B in the main text. We attribute this discrepancy to the excess charge due to the specific termination at the interface between the GaSb (001) substrate and the LuSb (001) film, as revealed by high-angle annular dark field scanning transmission electron microscopy (HAADF-STEM) of our thin films, shown in Fig. S10 and Fig. 5 in the main text. For the observed Ga-LuSb termination at the interface, we expect an excess charge of 1.5 electrons per 2D unit cell, to be accommodated in the interface states and/or transferred to the LuSb film, since the Fermi level of LuSb lies in the gap of GaSb.<sup>7</sup>

We note that the choice of using odd numbers of layers in the LuSb slab calculations, for instance 7, 13, 21, and 41ML shown in Fig. S7, instead of 6, 12, 20, and 40 in the experiments was to ensure inversion symmetry and facilitate the analysis of the band structures, and does not affect our results and conclusions. The results of a test calculation comparing the band structures of the slabs with 12 and 13 ML are shown in Fig. S8.

The estimated excess charge on the LuSb film is  $\sim 0.15 - 0.45$  electrons/2D unit cell, corresponding to 0.7-1 hole/2D unit cell (see discussions in the main text). Good agreement between the ARPES and DFT calculations is obtained after adding 0.25 electrons/2D unit cell to the LuSb slabs, as shown in Fig. 3C (main text), which corresponds to the observed 0.8 hole/2D unit at the interface band as measured in our transport measurements (see Fig. 4 in the main text). As a consequence of the charge transfer to the LuSb film we can see that the band minimum of the electron pocket at  $\bar{\Gamma}$  changes very slowly with respect to the Fermi level, while the size of the hole pocket at  $\bar{\Gamma}$  significantly decreases, in agreement with the ARPES measurements shown in Fig. 3B (main text). The variation of the size of the hole pocket at  $\bar{\Gamma}$  and band minimum of the electron pocket at  $\bar{\Gamma}$  as a function of the number of layers of LuSb is shown in Fig. S7.

Finally, in Fig. S9 we show that the existence of a two-dimensional hole gas at the LuSb/GaSb (001) interface does not depend on the LuSb surface, where we plotted the band structure of the LuSb/GaSb (001) superlattice with 17 ML of LuSb and 7 ML of GaSb, without a vacuum layer. The interface bands with Ga- $s$  character in LuSb/GaSb (001) superlattice are very similar to those obtained in the LuSb/GaSb/LuSb (001) slab calculation shown in Fig. 5 in the main text.

---

[1] Blöchl, P. Projector augmented-wave method. *Physical Review B* **50**, 17953 (1994).

[2] Kresse, G. & Hafner, J. Ab initio molecular dynamics for liquid metals. *Physical Review B* **47**, 558 (1993).

- [3] Kresse, G. & Hafner, J. Ab initio molecular-dynamics simulation of the liquid-metal–amorphous-semiconductor transition in germanium. *Physical Review B* **49**, 14251 (1994).
- [4] Perdew, J. P., Burke, K. & Ernzerhof, M. Generalized gradient approximation made simple. *Physical Review Letters* **77**, 3865 (1996).
- [5] Heyd, J., Scuseria, G. E. & Ernzerhof, M. Hybrid functionals based on a screened Coulomb potential. *Journal of Chemical Physics* **118**, 8207–8215 (2003).
- [6] Heyd, J., Scuseria, G. E. & Ernzerhof, M. Erratum: “Hybrid functionals based on a screened Coulomb potential” [J. Chem. Phys. 118, 8207 (2003)]. *Journal of Chemical Physics* **124**, 219906 (2006).
- [7] Khalid, S., Sharan, A. & Janotti, A. Hybrid functional calculations of electronic structure and carrier densities in rare-earth monpnictides. *Physical Review B* **101**, 125105 (2020).
- [8] Chatterjee, S. *et al.* Weak antilocalization in quasi-two-dimensional electronic states of epitaxial LuSb thin films. *Physical Review B* **99**, 125134 (2019).
- [9] Bharathan, J., Narayan, J., Rozgonyi, G. & Bulman, G. E. Poisson ratio of epitaxial germanium films grown on silicon. *Journal of electronic materials* **42**, 40–46 (2013).
- [10] Mir, S. H. *et al.* Static and dynamical properties of heavy actinide monpnictides of lutetium. *Scientific reports* **6**, 29309 (2016).

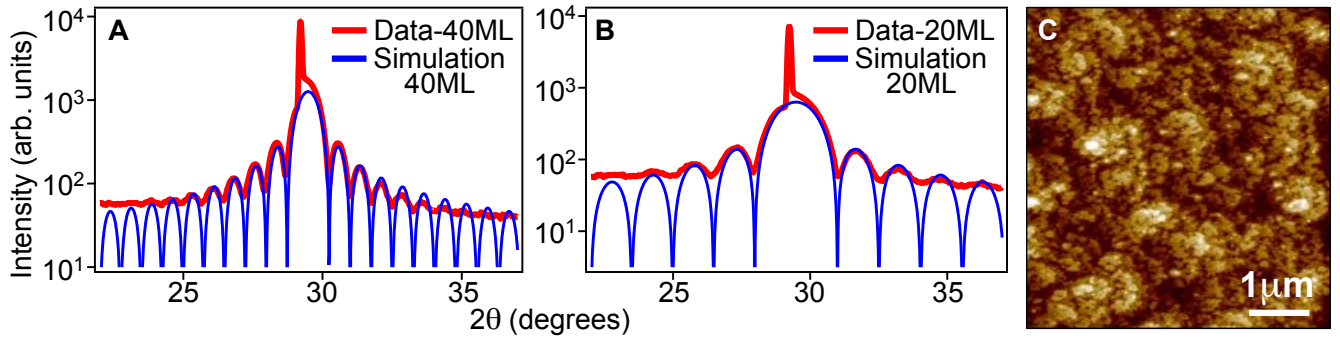

FIG. S1. **Structural characterization of LuSb/GaSb thin films** Out-of-plane  $\theta - 2\theta$  x-ray diffraction scans around the LuSb (002) Bragg peak showing Laue oscillations for the (A) 40ML and (B) 20ML thick films along with the corresponding fits, which show excellent agreement. (C) Atomic force microscopy (AFM) image of a 6ML thick film confirming that our thin films are uniform over a wide area even in the ultra-thin limit with an RMS roughness of 0.2 nm over a  $5\mu\text{m} \times 5\mu\text{m}$  field of view.

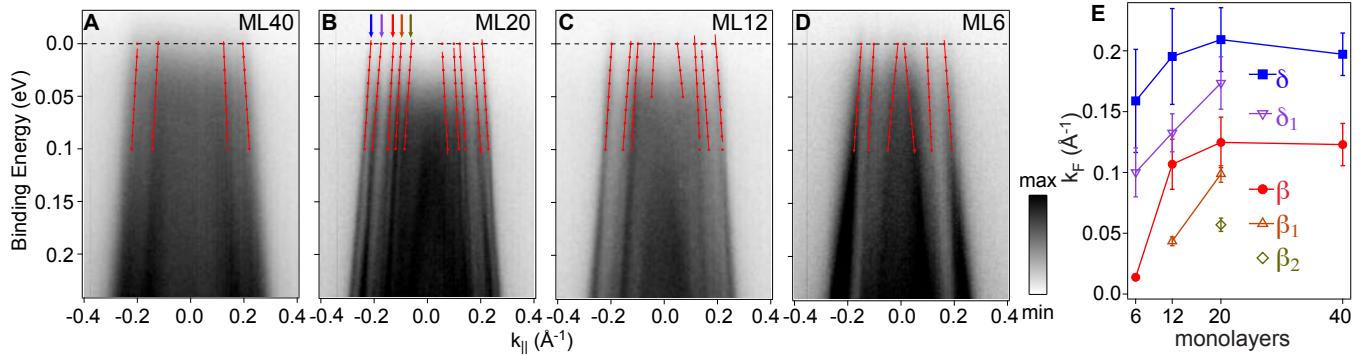

FIG. S2. **Extraction of Fermi wavevector ( $k_F$ ) from the ARPES data.** ARPES data along  $\bar{M} - \Gamma - \bar{M}$  at the bulk  $\Gamma$  point taken at 70K for the (A) 40ML (B) 20ML (C) 12ML (D) 6ML thick films. Extracted dispersions and corresponding fits are shown in red. (E) Extracted Fermi wavevectors ( $k_F$ ) as a function of film thickness. Arrows in B indicate the quantum well states, thickness dependencies of which are plotted in E.

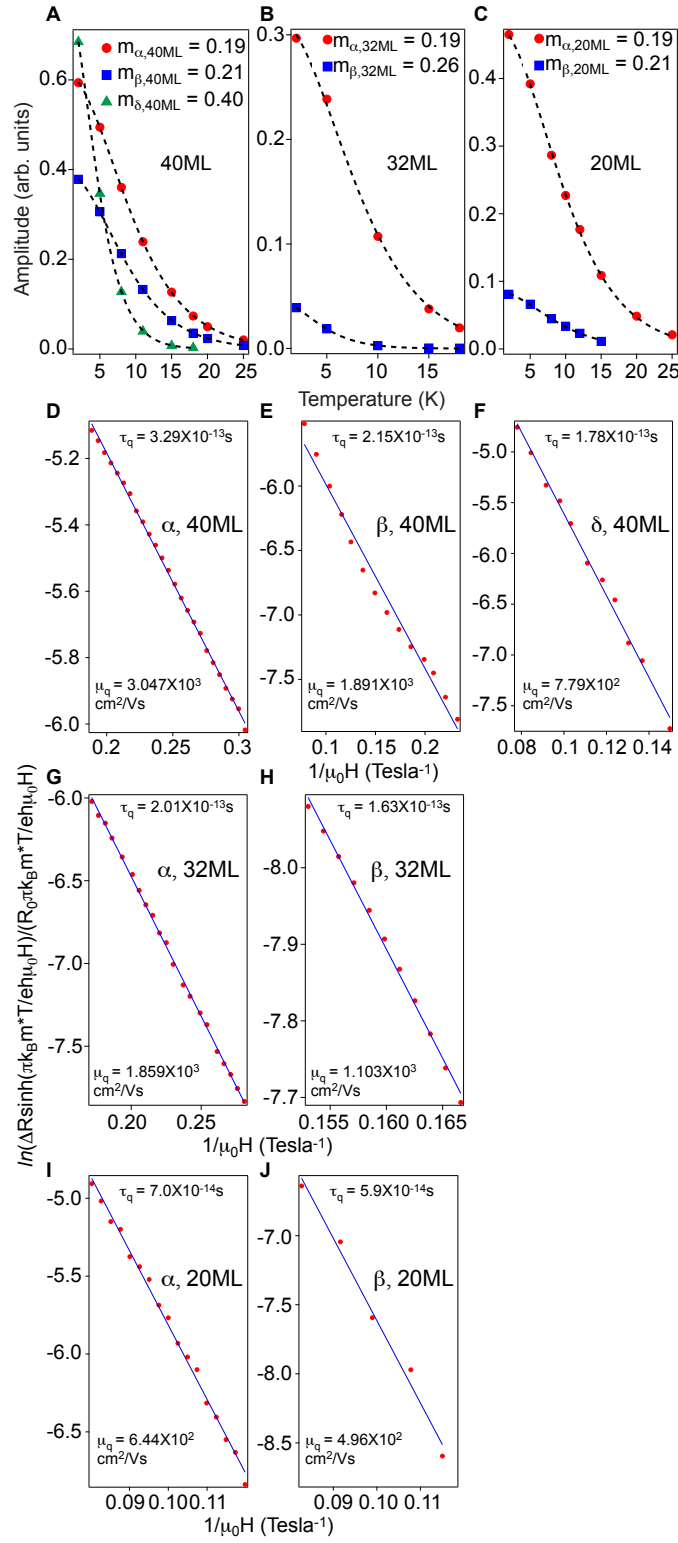

FIG. S3. **Effective mass and quantum mobility of carriers in LuSb thin films** Effective mass calculated from the quantum oscillation measurements for the (A) 40ML (B) 32ML (C) 20ML thick film. Quantum mobility is calculated from the linear slope of the fits for the (D)  $\alpha$  (E)  $\beta$  (F)  $\delta$  Fermi pocket for the 40ML thick film, (G)  $\alpha$  (H)  $\beta$  pocket for the 32ML, (I)  $\alpha$  (J)  $\beta$  pocket for the 20ML thick film. Quantum mobility ( $\mu_q$ ) and corresponding lifetime ( $\tau_q$ ) values are marked in the corresponding panels.

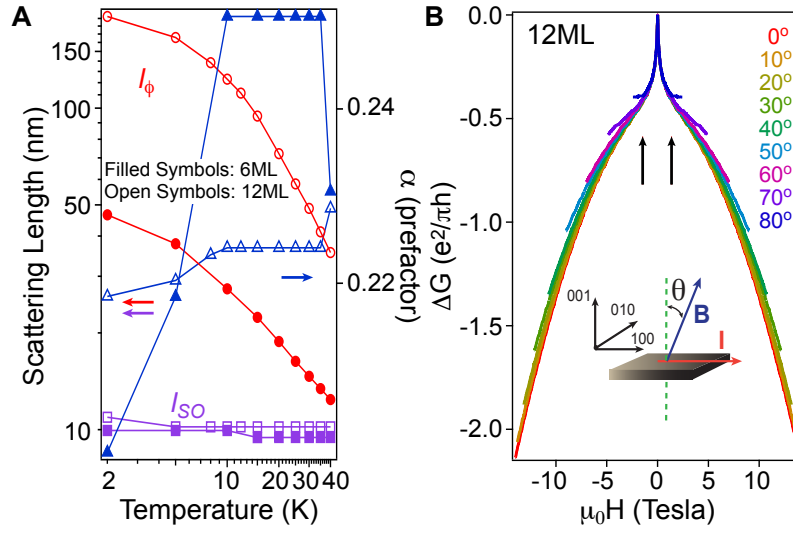

FIG. S4. **Quantum corrections to the transport data in ultra-thin LuSb thin films** (A) Phase coherence and spin-orbit scattering lengths as a function of temperature for both the 12 and 6ML thick films. While the phase coherence length is reduced significantly at higher temperatures the spin-orbit scattering length roughly remains independent of temperature. (B) Angle-dependent magnetoresistance data for the 12ML thick film showing angular scaling behavior expected from a two-dimensional electronic system between magnetic fields of  $\pm 1$  Tesla.

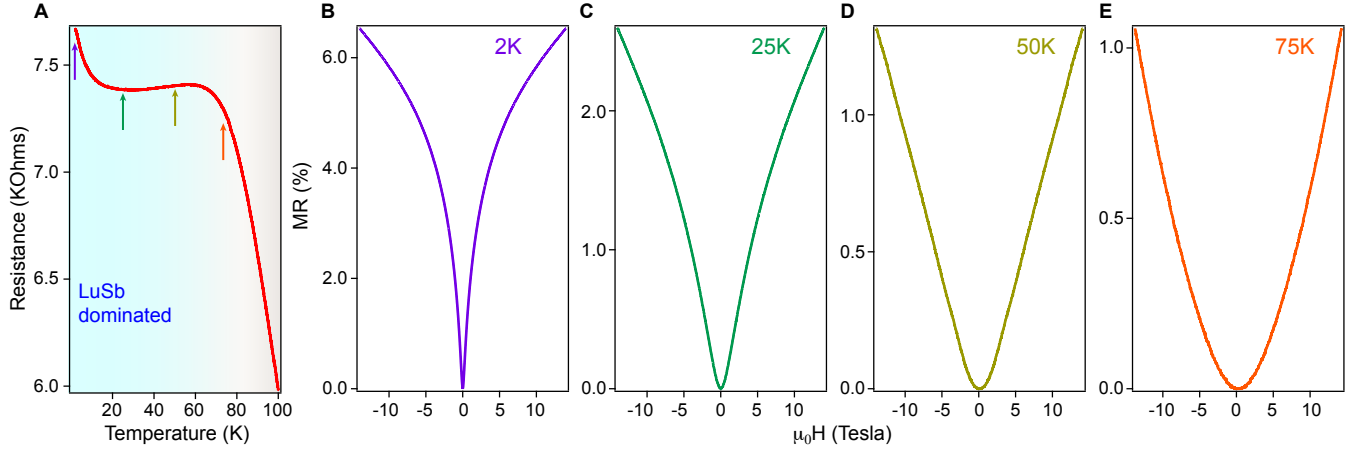

FIG. S5. **Evolution of magnetoresistance with temperature in the 6ML thick LuSb thin films.** (A) Temperature dependence of resistance of the 6ML thick film. Temperature region dominated by LuSb atomic layers when carriers from the underlying GaSb layers freeze out is highlighted in blue. Magnetoresistance behavior at (B) 2K (C) 25K (D) 50K (E) 75K. Temperatures at which magnetoresistance data is obtained are highlighted in panel A. At higher temperatures magnetoresistance evolves from a saturating behavior to a non-saturating behavior, as seen in the thicker films underscoring the importance of electron-electron interaction effects in modifying magnetoresistance behavior at low temperatures in few atomic layer geometries.

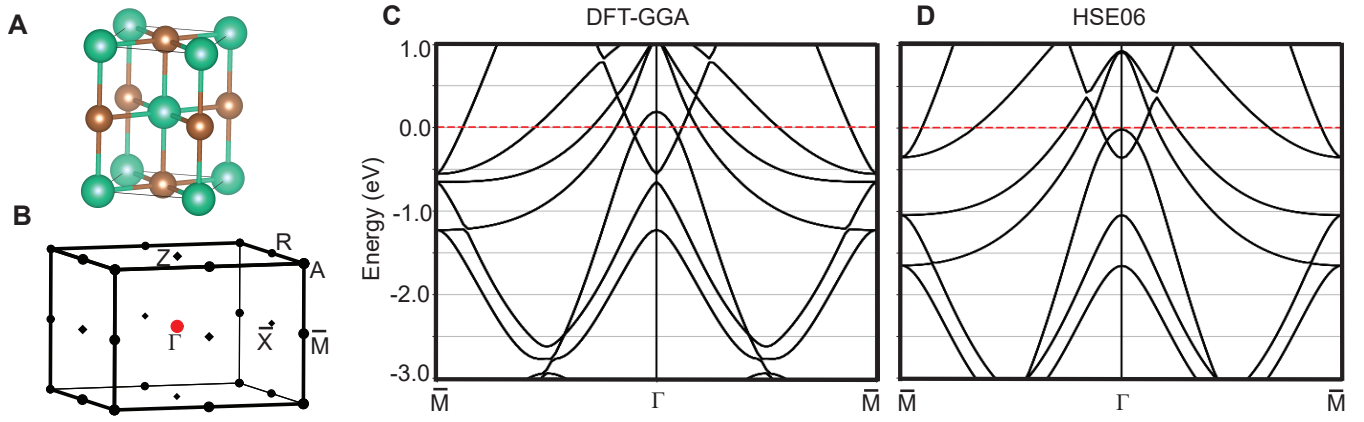

FIG. S6. **Electronic band structure of bulk LuSb for the 4 atom tetragonal cell.** (A) Four atom tetragonal unit cell. (B) Brillouin zone. Calculations made using the (C) DFT-GGA and (D) HSE06 functional. In DFT-GGA, the overlap between the electron and hole pockets are significantly overestimated leading to an overestimation of the carrier density. The carrier density using the HSE06 functional is in good agreement with the experimental data.<sup>8</sup>

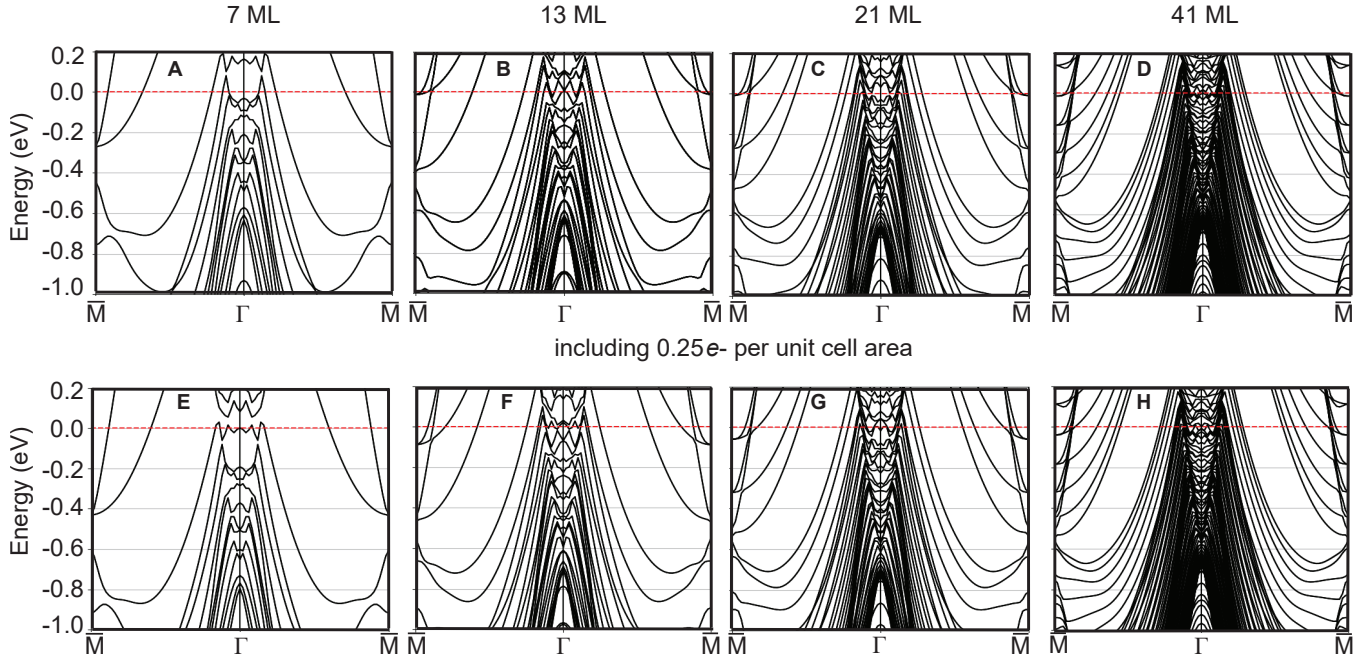

FIG. S7. **Calculated electronic structure of free-standing LuSb (001) films as a function of film thickness (number of monolayers or ML)** for (A) 7ML, (B) 13ML, (C) 21ML, and (D) 41ML. Corresponding electronic structure of LuSb (001) films in (E)-(H) after adding 0.25 electrons per unit cell area to account for the excess charge at the interface between Ga terminated GaSb (001) and LuSb (001) atomic layers.

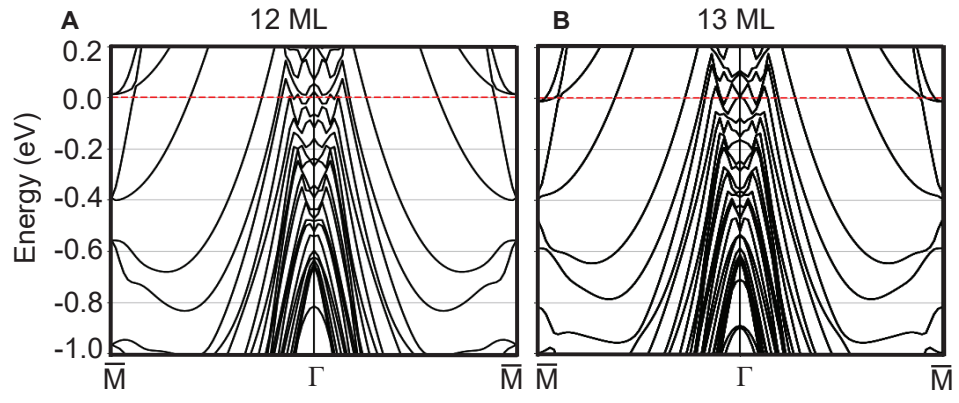

FIG. S8. Calculated electronic structure of free-standing LuSb (001) films for (A) 12ML, (B) 13ML.

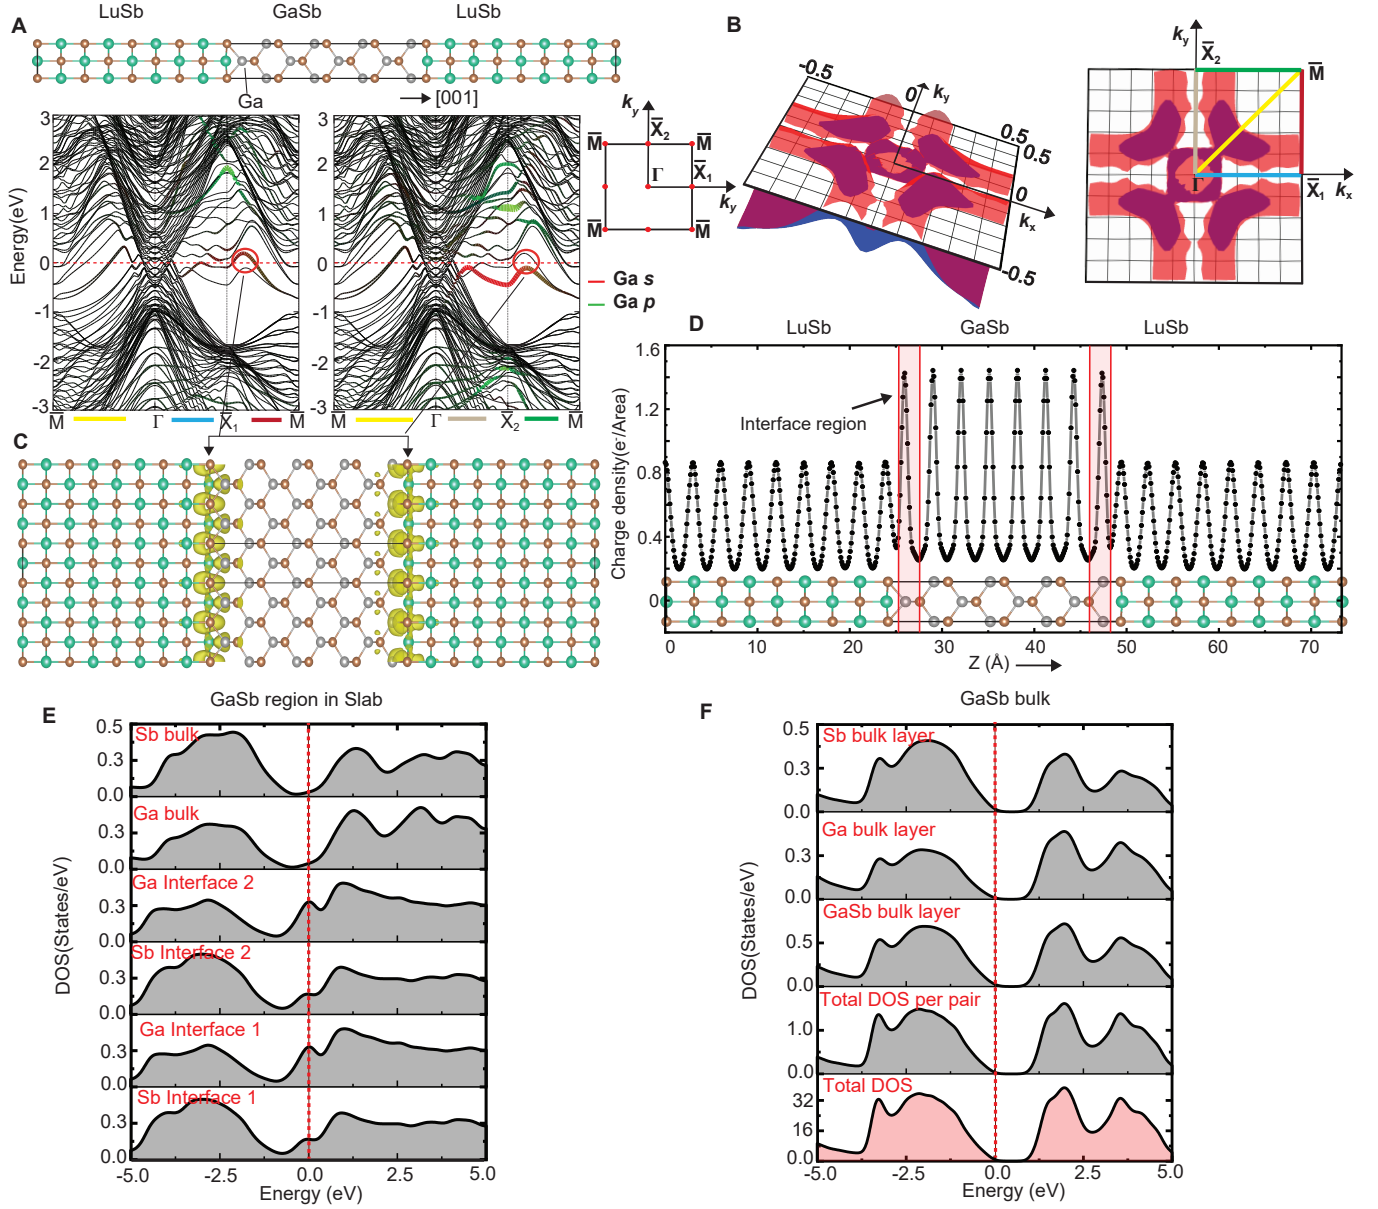

FIG. S9. **Origin of the two-dimensional hole gas at a rock salt/zincblende interface.** Electronic structure of a LuSb/GaSb/LuSb (001) slab showing (A) Interface bands that originates from  $s$  orbital of the Ga atom at the interface; (B) 3D view of the two interface bands associated with the two equivalent interfaces, yet rotated, the structure used in the simulation. (C) Charge density distribution of the single-particle state at the maximum of the hole band crossing the Fermi level along the  $\bar{X}_2$ - $\bar{M}$  direction. (D) Valence charge density distribution of the LuSb/GaSb/LuSb (001) slab along the direction perpendicular to the interface. (E) Density of states (DOS) calculation for the GaSb region in the LuSb/GaSb/LuSb (001) slab. (F) Density of states (DOS) calculation for the GaSb bulk.

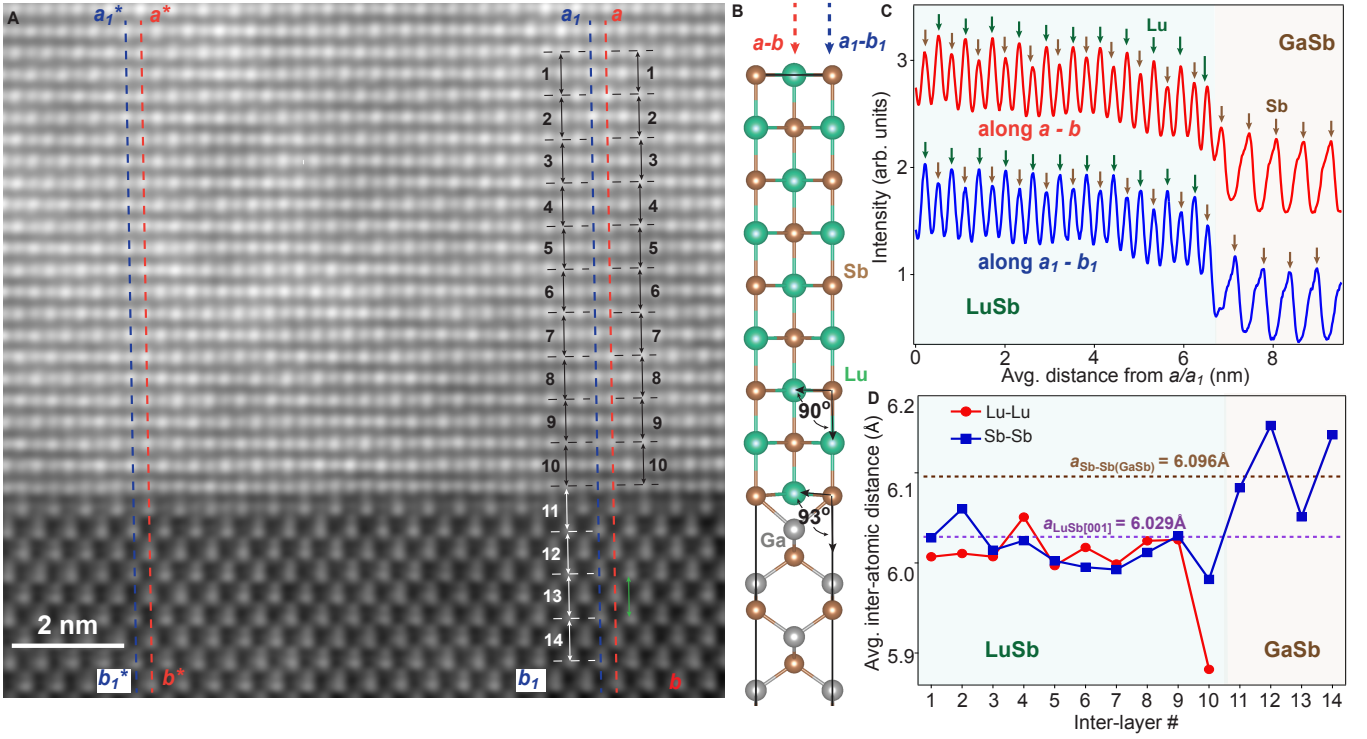

FIG. S10. **Structural distortion of the Lu atoms at the LuSb/GaSb interface** (A) HAADF-STEM image along [110] zone-axis. The data has been Fourier filtered for clarity. (B) A ball-and-stick model of the proposed atomic arrangement showing two different atomic columns, one which is terminated with a Lu atom on the LuSb side at the interface ( $a-b$ ), and the other terminated with an Sb atom ( $a_1-b_1$ ). Lu atoms are distorted at the interface shown by the different values of the bond angles. (C) Intensity profiles along line scans, shown in **A**, obtained by averaging along ( $a-b$ ) between ( $a-b$ ) and ( $a^*-b^*$ ) (red line) and along ( $a_1-b_1$ ) between ( $a_1-b_1$ ) and ( $a_1^*-b_1^*$ ) (blue line). (D) Evolution of the Lu-Lu inter-atomic distances along the columns ( $a-b$ ) and between Sb-Sb along the columns ( $a_1-b_1$ ). Lu-Lu inter-atomic distance in the out-of-plane direction [001] is smaller at the interface, which is absent for the Sb-Sb case, consistent with the predicted interfacial buckling model in **B**. Observed value of the Lu-Lu inter-atomic distance is found to be in agreement with the expected out-of-plane LuSb lattice constant (violet dotted line) for a pseudomorphic LuSb film on GaSb substrate<sup>9</sup> and a LuSb Poisson's ratio of 0.24.<sup>10</sup>
